# Supplementary material for: On the Provable Advantage of Unsupervised Pretraining
Source: arXiv:2303.01566 source file (2023-03-02)
Supplement: Supplementary file 1 [file Appendix.tex]

\section{Appendix}
